# Supplementary material for: Physiology-Aware Masked Cross-Modal Reconstruction for Biosignal Representation Learning
Source: arXiv:2605.00973 source file (2026-05-01)
Supplement: Supplementary file 1 [file mimic3.tex]

\section{Justification of Generalization from Lab-to-Wearable Datasets}\label{app:mimic3}

During pretraining, ECG provides a precise temporal reference that aligns each heartbeat with the onset of the corresponding PPG pulse. This supervision teaches {\name} to organize PPG representations around beat-level timing rather than raw signal samples. During most evaluations, ECG is no longer required because the model has learned how beat timing manifests in the PPG waveform itself. 
% Our findings on the transferability of PPG representations across devices and subjects are consistent with prior work~\cite{pulseppg, papagei}, which shows that models pretrained on clinical datasets can generalize to wearable data and achieve performance comparable to models trained in the reverse direction (Table~\ref{tab:open_source}). Overall, we believe that {\name} can extend the pretraining corpus for wearable biosignal representation learning to include more diverse and generic data sources.
Our observations of cross-device and cross-subject transferability are consistent with prior work~\cite{pulseppg, papagei}, which demonstrates that representations pretrained on clinical datasets also can generalize to wearable data, achieving performance comparable to models pretrained in the reverse direction. Together, these findings suggest that clinically sourced ECG–PPG co-training provides physiologically grounded supervision that is not device-specific. Overall, we believe that {\name} enables the pretraining corpus for wearable biosignal representation learning to be extended toward more diverse, heterogeneous, and generic data sources.

% Although PPG waveforms may differ in shape or amplitude across individuals and sensing devices, the temporal order of rise, peak, and decay remains consistent.

% Importantly, this timing structure serves as a proxy for many downstream health tasks, since changes in cardiovascular state often appear as changes in beat timing and pulse dynamics rather than absolute waveform shape~\cite{pat}. 

% As a result, {\name} can infer meaningful and task-relevant information directly from PPG alone, enabling robust generalization to wearable signals, even pretrained on MIMIC-III.
